# Supplementary material for: Assessing the alignment between the information needs of developers and the documentation of programming languages: A case study on Rust
Source: arXiv:2202.04431 source file (2022-02-08)
Supplement: Supplementary file 1 [file apx-supp-mat.tex]

\section{Supplementary Material}
\label{apx:supp-mat}

A supplementary material containing the data used in our study of the conceptual aligment of \rust documentation is available at \url{}.
